# Supplementary material for: Systematic Literature Review of AI-enabled Spectrum Management in 6G and Future Networks
Source: arXiv:2407.10981 source file (2024-06-12)
Supplement: Supplementary file 1 [file appendix.tex]

\newpage
\setcounter{table}{0}

\footnotesize  % Switch from 12pt to 11pt; otherwise, table won't fit
% % default: \fill
 \setlength{\LTleft}{0pt plus 1fill minus 1fill}%
 % \setlength{\LTright}{\LTleft}
 % \setlength{\tabcolsep}{2pt}
 % \bushra{To be Removed once the Link is placed in Sharepoint, Also will used [36] then. }
\begin{longtable}{|p{0.05cm}|m{4cm}|m{4cm}|m{3cm}|p{0.05cm}|}
\caption{Selected studies in the review. Here ID denotes study identification number.} \label{appendix} \\

\hline \multicolumn{1}{|c|}{\textbf{ID}} & \multicolumn{1}{c|}{\textbf{Title}} & \multicolumn{1}{c|}{\textbf{Authors}} &
\multicolumn{1}{c|}{\textbf{Venue}} &
\multicolumn{1}{c|}{\textbf{Year}}
 \\ \hline 
\endfirsthead
\multicolumn{5}{c}%
{{\bfseries Appendix\  A\ -- continued from previous page}} \\
\hline \multicolumn{1}{|c|}{\textbf{ID}} & \multicolumn{1}{c|}{\textbf{Title}} & \multicolumn{1}{c|}{\textbf{Authors}} &
\multicolumn{1}{c|}{\textbf{Venue}} &
\multicolumn{1}{c|}{\textbf{Year}} 
\endhead
\hline \multicolumn{5}{|c|}{{Continued on next page}} \\ \hline
\endfoot
\hline
\endlastfoot
\hline
S1&RF-Sensing: A New Way to Observe Surroundings&Khunteta, Shubham, Saikrishna, Pedamalli, Agrawal, Avani, Kumar, Ashwini, Chavva, Ashok Kumar Reddy&IEEE Access&2022 \\ \hline
S2&Dynamic spectrum allocation following machine learning-based traffic predictions in 5G&Rony, Rakibul Islam, Lopez-Aguilera, Elena, Garcia-Villegas, Eduard&IEEE Access&2021 \\ \hline
S3&Confidence aware deep learning driven wireless resource allocation in shared spectrum bands&Ganewattha, Chanaka, Khan, Zaheer, Latva-Aho, Matti, Lehtoma&IEEE Access&2022 \\ \hline
S4&Secure Industrial IoT Systems via RF Fingerprinting Under Impaired Channels With Interference and Noise&Gul, Omer Melih, Kulhandjian, Michel, Kantarci, Burak, Touazi, Azzedine, Ellement, Cliff, D’amours, Claude&IEEE Access&2023 \\ \hline
S5&GPDS: A multi-agent deep reinforcement learning game for anti-jamming secure computing in MEC network&Chen, Miaojiang, Liu, Wei, Zhang, Ning, Li, Junling, Ren, Yingying, Yi, Meng, Liu, Anfeng&Expert Systems with Applications&2022 \\ \hline
S6&Generalized wireless adversarial deep learning&Restuccia, Francesco, D'Oro, Salvatore, Al-Shawabka, Amani, Rendon, Bruno Costa, Chowdhury, Kaushik, Ioannidis, Stratis, Melodia, Tommaso&Computer Networks&2020 \\ \hline
S7&Cybertwin-driven resource allocation using deep reinforcement learning in 6G-enabled edge environment&Jain, Vibha, Kumar, Bijendra, Gupta, Aditya&Journal of King Saud University – Computer and Information Sciences&2022 \\ \hline
S8&Online edge learning offloading and resource management for UAV-assisted MEC secure communications&Ding, Yu, Feng, Yunqi, Lu, Weidang, Zheng, Shilian, Zhao, Nan, Meng, Limin, Nallanathan, Arumugam, Yang, Xiaoniu& IEEE Journal of Selected Topics in Signal Processing&2022 \\ \hline
S9&When deep reinforcement learning meets federated learning: Intelligent multi-timescale resource management for multi-access edge computing in 5G ultradense network&Yu, Shuai, Chen, Xu, Zhou, Zhi, Gong, Xiaowen, Wu, Di&IEEE Internet of Things Journal&2020 \\ \hline
S10&Federated Reinforcement Learning-Based Resource Allocation for D2D-Aided Digital Twin Edge Networks in 6G Industrial IoT&Guo, Qi, Tang, Fengxiao, Kato, Nei&IEEE Transactions on Industrial Informatics&2022 \\ \hline
S11&Reinforcement learning based latency minimization in secure NOMA-MEC systems with hybrid SIC&Wang, Kaidi, Li, Haodong, Ding, Zhiguo, Xiao, Pei&IEEE Transactions on Wireless Communications&2022 \\ \hline
S12&Security Hardening of Intelligent Reflecting Surfaces Against Adversarial Machine Learning Attacks&Catak, Ferhat Ozgur, Kuzlu, Murat, Tang, Haolin, Catak, Evren, Zhao, Yanxiao&IEEE Access&2022 \\ \hline
S13&Beyond 5G for digital twins of UAVs&Lv, Zhihan, Chen, Dongliang, Feng, Hailing, Lou, Ranran, Wang, Huihui&Computer Networks&2021 \\ \hline
S14&A variational autoencoder-based secure transceiver design using deep learning&Lin, Chia-Hung, Wu, Chao-Chin, Chen, Kuan-Fu, Lee, Ta-Sung&IEEE GLOBECOM&2020 \\ \hline

S15&The Hexa-X project vision on Artificial Intelligence and Machine Learning-driven Communication and Computation co-design for 6G&Merluzzi, Mattia, Borsos, Tams, Rajatheva, Nandana, Benczr, Andrs A, Farhadi, Hamed, Yassine, Taha, Mu&IEEE Access&2023 \\ \hline
S16&Multi-UAV-assisted computation offloading in DT-based networks: A distributed deep reinforcement learning approach&Shi, Junling, Li, Chunyu, Guan, Yunchong, Cong, Peiyu, Li, Jie&Computer Communications&2023 \\ \hline
S17&Mitigating Jamming Attack in 5G Heterogeneous Networks: A Federated Deep Reinforcement Learning Approach&Sharma, Himanshu, Kumar, Neeraj, Tekchandani, Rajkumar&IEEE Transactions on Vehicular Technology&2022 \\ \hline
S18 & Exploring Practical Vulnerabilities of Machine Learning-based Wireless Systems & Liu, Zikun, Xu, Changming, Sie, Emerson, Singh, Gagandeep, Vasisht, Deepak & USENIX Symposium on Networked Systems Design and Implementation & 2023  \\ \hline
S19&Digital Twin-Aided Learning for Managing Reconfigurable Intelligent Surface-Assisted, Uplink, User-Centric Cell-Free Systems&Cui, Yingping, Lv, Tiejun, Ni, Wei, Jamalipour, Abbas&IEEE Journal on Selected Areas in Communications&2023 \\ \hline
S20&mmecho: A mmwave-based acoustic eavesdropping method&Hu, Pengfei, Li, Wenhao, Spolaor, Riccardo, Cheng, Xiuzhen&IEEE Symposium on Security and Privacy&2023 \\ \hline
S21&A D2D-Aided Federated Learning Scheme With Incentive Mechanism in 6G Networks&Fantacci, Romano, Picano, Benedetta&IEEE Access&2022 \\ \hline
S22&Joint resource allocation to minimize execution time of federated learning in cell-free massive MIMO&Vu, Tung Thanh, Ngo, Duy Trong, Ngo, Hien Quoc, Dao, Minh Ngoc, Tran, Nguyen Hoang, Middleton, Richard H&IEEE Internet of Things Journal&2022 \\ \hline
S23&Joint resource management for mobility supported federated learning in Internet of Vehicles&Wang, Ge, Xu, Fangmin, Zhang, Hengsheng, Zhao, Chenglin&Future Generation Computer Systems&2022 \\ \hline
S24&Mitigating attacks on artificial intelligence-based spectrum sensing for cellular network signals&Catak, Ferhat Ozgur, Kuzlu, Murat, Sarp, Salih, Catak, Evren, Cali, Umit&IEEE GLOBECOM&2022 \\ \hline
S25&Privacy-preserving federated k-means for proactive caching in next generation cellular networks&Liu, Yang, Ma, Zhuo, Yan, Zheng, Wang, Zhuzhu, Liu, Ximeng, Ma, Jianfeng&Journal of King Saud University – Computer and Information Sciences&2020 \\ \hline
S26&Resource allocation and device pairing for energy-efficient NOMA-enabled federated edge learning&Hu, Youqiang, Huang, Hejiao, Yu, Nuo&Computer Communications&2023 \\ \hline
S27&Adaptive resource reservation to survive against adversarial resource selection jamming attacks in 5g nr-v2x distributed mode 2&Djaidja, Taki Eddine Toufik, Brik, Bouziane, Senouci, Sidi Mohammed, Ghamri-Doudane, Yacine&IEEE International Conference on Communications&2022 \\ \hline
S28&Securing radio resources allocation with deep reinforcement learning for IoE services in next-generation wireless networks&Peng, Yuhuai, Xue, Xiaojing, Bashir, Ali Kashif, Zhu, Xiaogang, Al-Otaibi, Yasser D, Tariq, Usman, Yu, Keping&IEEE Transactions on Network Science and Engineering&2022 \\ \hline
S29&A deep convolutional neural network based transfer learning method for non-cooperative spectrum sensing&Pati, Bipun Man, Kaneko, Megumi, Taparugssanagorn, Attaphongse&IEEE Access&2020 \\ \hline
S30&Spectrum Sensing in Cognitive Radio Using CNN-RNN and Transfer Learning&Solanki, Surendra, Dehalwar, Vasudev, Choudhary, Jaytrilok, Kolhe, Mohan Lal, Ogura, Koki&IEEE Access&2022 \\ \hline
S31&When attackers meet AI: Learning-empowered attacks in cooperative spectrum sensing&Luo, Zhengping, Zhao, Shangqing, Lu, Zhuo, Xu, Jie, Sagduyu, Yalin E&IEEE Transactions on Mobile Computing&2020 \\ \hline
S32&Adversarial deep learning for over-the-air spectrum poisoning attacks&Sagduyu, Yalin E, Shi, Yi, Erpek, Tugba&IEEE Transactions on Mobile Computing&2019 \\ \hline
S33&Channel-aware adversarial attacks against deep learning-based wireless signal classifiers&Kim, Brian, Sagduyu, Yalin E, Davaslioglu, Kemal, Erpek, Tugba, Ulukus, Sennur&IEEE Transactions on Wireless Communications&2021 \\ \hline
S34&Deep learning driven physical layer security for a simultaneously wireless information and power transfer network&Li, Junxia, Zhao, Hui, Huang, Yiyun, Zhang, Miao, Lal, Sujesh P&Alexandria Engineering Journal&2022 \\ \hline
S35&Threshold-free physical layer authentication based on machine learning for industrial wireless CPS&Pan, Fei, Pang, Zhibo, Wen, Hong, Luvisotto, Michele, Xiao, Ming, Liao, Run-Fa, Chen, Jie&IEEE Transactions on Industrial Informatics&2019 \\ \hline
S36&Improving medium access efficiency with intelligent spectrum learning&Yang, Bo, Cao, Xuelin, Omotere, Oluwaseyi, Li, Xiangfang, Han, Zhu, Qian, Lijun&IEEE Access&2020 \\ \hline
S37&Signal detection and classification in shared spectrum: A deep learning approach&Zhang, Wenhan, Feng, Mingjie, Krunz, Marwan, Abyaneh, Amir Hossein Yazdani&IEEE INFOCOM&2021 \\ \hline
S38&A Radio Frequency Region-of-Interest Convolutional Neural Network for Wideband Spectrum Sensing&Olesiski, Adam, Piotrowski, Zbigniew&Sensors&2023 \\ \hline
S39&Charm: Nextg spectrum sharing through data-driven real-time o-ran dynamic control&Baldesi, Luca, Restuccia, Francesco, Melodia, Tommaso&IEEE INFOCOM&2022 \\ \hline
S40&Learning the unknown: Improving modulation classification performance in unseen scenarios&Perenda, Erma, Rajendran, Sreeraj, Bovet, Gerome, Pollin, Sofie, Zheleva, Mariya&IEEE INFOCOM&2021 \\ \hline
S41&A deep reinforcement learning framework for spectrum management in dynamic spectrum access&Song, Hao, Liu, Lingjia, Ashdown, Jonathan, Yi, Yang&IEEE Internet of Things Journal&2021 \\ \hline
S42&End-to-end learning from spectrum data: A deep learning approach for wireless signal identification in spectrum monitoring applications&Kulin, Merima, Kazaz, Tarik, Moerman, Ingrid, De Poorter, Eli&IEEE Access&2018 \\ \hline
S43&Deep learning-based spectrum prediction collision avoidance for hybrid wireless environments&Mennes, Ruben, Claeys, Maxim, De Figueiredo, Felipe AP, Jabandvz&IEEE Access&2019 \\ \hline
S44&An ai-based incumbent protection system for collaborative intelligent radio networks&Camelo, Miguel, Mennes, Ruben, Shahid, Adnan, Struye, Jakob, Donato, Carlos, Jabandzic, Irfan, Giannoulis, Spilios, Mahfoudhi, Farouk, Maddala, Prasanthi, Seskar, Ivan, others&IEEE Wireless Communications&2020 \\ \hline
S45&Optimizing primary user privacy in spectrum sharing systems&Clark, Matthew, Psounis, Konstantinos& IEEE/ACM Transactions on Networking &2020 \\ \hline
S46&Pattern-aware intelligent anti-jamming communication: A sequential deep reinforcement learning approach&Liu, Songyi, Xu, Yifan, Chen, Xueqiang, Wang, Ximing, Wang, Meng, Li, Wen, Li, Yangyang, Xu, Yuhua&IEEE Access&2019 \\ \hline
S47&“jam me if you can:” defeating jammer with deep dueling neural network architecture and ambient backscattering augmented communications&Van Huynh, Nguyen, Nguyen, Diep N, Hoang, Dinh Thai, Dutkiewicz, Eryk&IEEE Journal on Selected Areas in Communications&2019 \\ \hline
S48&DeepFake: Deep dueling-based deception strategy to defeat reactive jammers&Van Huynh, Nguyen, Hoang, Dinh Thai, Nguyen, Diep N, Dutkiewicz, Eryk&IEEE Transactions on Wireless Communications&2021 \\ \hline
S49&CyberSpec: Behavioral Fingerprinting for Intelligent Attacks Detection on Crowdsensing Spectrum Sensors&Celdrn, Alberto Huertas, Snchez, Pedro Miguel Snchez, Bovet, Gro& IEEE Transactions on Dependable and Secure Computing&2023 \\ \hline
S50&Differential privacy and IRS empowered intelligent energy harvesting for 6G Internet of Things&Pan, Qianqian, Wu, Jun, Zheng, Xi, Yang, Wu, Li, Jianhua&IEEE Internet of Things Journal&2021 \\ \hline
S51&Federated learning for intelligent transmission with space-air-ground integrated network (SAGIN) toward 6G&Tang, Fengxiao, Wen, Cong, Chen, Xuehan, Kato, Nei&IEEE Network&2022 \\ \hline
S52&Federated Multi-Agent Deep Reinforcement Learning (Fed-MADRL) for Dynamic Spectrum Access&Chang, Hao-Hsuan, Song, Yifei, Doan, Thinh T, Liu, Lingjia&IEEE Transactions on Wireless Communications&2023 \\ \hline
S53&How effective is the artificial noise? Real-time analysis of a PHY security scenario&Goekceli, Selahattin, Cepheli, Oezge, Basaran, Semiha Tedik, Kurt, Guenes Karabulut, Dartmann, Guido, Ascheid, Gerd&IEEE GLOBECOM&2017 \\ \hline
S54&Anomaly detection based on multidimensional data processing for protecting vital devices in 6G-enabled massive IIoT&Han, Guangjie, Tu, Juntao, Liu, Li, Martnez-Garca, Miguel, Peng, Yan& IEEE Internet of Things Journal&2021 \\ \hline
S55&Self-Optimizing Data Offloading in Mobile Heterogeneous Radio-Optical Networks: A Deep Reinforcement Learning Approach&Shao, Sihua, Nazzal, Mahmoud, Khreishah, Abdallah, Ayyash, Moussa&IEEE Network&2022 \\ \hline
S56&Defensive distillation-based adversarial attack mitigation method for channel estimation using deep learning models in next-generation wireless networks&Catak, Ferhat Ozgur, Kuzlu, Murat, Catak, Evren, Cali, Umit, Guler, Ozgur&IEEE Access&2022 \\ \hline
S57&Data-augmentation-based cellular traffic prediction in edge-computing-enabled smart city&Wang, Zi, Hu, Jia, Min, Geyong, Zhao, Zhiwei, Wang, Jin&IEEE Transactions on Industrial Informatics&2020 \\ \hline
S58&Federated learning for 5G base station traffic forecasting&Perifanis, Vasileios, Pavlidis, Nikolaos, Koutsiamanis, Remous-Aris, Efraimidis, Pavlos S&Computer Networks&2023 \\ \hline
S59&A self-adaptive deep learning-based system for anomaly detection in 5G networks&Maim, Lorenzo Fernndez, Gmez, ngel Luis Perales, Clemente, Flix J Garca, Prez, Manuel Gil, Prez, Gregorio Martnez&IEEE Access&2018 \\ \hline
S60&Anomaly detection approach for urban sensing based on credibility and time-series analysis optimization model&Zhang, Hong, Li, Zhanming&IEEE Access&2019 \\ \hline
S61&Fault-tolerant event region detection on trajectory pattern extraction for industrial wireless sensor networks&Liu, Li, Han, Guangjie, He, Yu, Jiang, Jinfang&IEEE Transactions on Industrial Informatics&2019 \\ \hline
S62&Context-and-social-aware online beam selection for mmwave vehicular communications&Li, Dapeng, Wang, Shichao, Zhao, Haitao, Wang, Xiaoming&IEEE Internet of Things Journal&2020 \\ \hline
S63&Machine learning enabling analog beam selection for concurrent transmissions in millimeter-wave V2V communications&Yang, Yang, Gao, Zhen, Ma, Yao, Cao, Biao, He, Dazhong&IEEE Transactions on Vehicular Technology&2020  \\ \hline
S64&Computer vision aided mmWave beam alignment in V2X communications&Xu, Weihua, Gao, Feifei, Tao, Xiaoming, Zhang, Jianhua, Alkhateeb, Ahmed&IEEE Transactions on Wireless Communications&2022 \\ \hline
S65&A deep learning-based low overhead beam selection in mmWave communications&Echigo, Haruhi, Cao, Yuwen, Bouazizi, Mondher, Ohtsuki, Tomoaki&IEEE Transactions on Vehicular Technology&2021 \\ \hline
S66&Deep learning-based mmWave beam selection for 5G NR/6G with sub-6 GHz channel information: Algorithms and prototype validation&Sim, Min Soo, Lim, Yeon-Geun, Park, Sang Hyun, Dai, Linglong, Chae, Chan-Byoung&IEEE Access &2020 \\ \hline
S67&Deep learning for mmWave beam and blockage prediction using sub-6 GHz channels&Alrabeiah, Muhammad, Alkhateeb, Ahmed&IEEE Transactions on Communications&2020 \\ \hline
S68&LIDAR data for deep learning-based mmWave beam-selection&Klautau, Aldebaro, Gonzlez-Prelcic, Nuria, Heath, Robert W&IEEE Transactions on Communications &2019 \\ \hline
S69&Deep scanning—beam selection based on deep reinforcement learning in massive mimo wireless communication system&Kim, Minhoe, Lee, Woongsup, Cho, Dong-Ho&Electronics&2020 \\ \hline
S70&Fast specific absorption rate aware beamforming for downlink SWIPT via deep learning&Zhang, Juping, Zheng, Gan, Krikidis, Ioannis, Zhang, Rui&IEEE GLOBECOM&2020 \\ \hline
S71&A two-step neural network based beamforming in MIMO without reference signal&Zhao, Yuyan, Liu, Yanan, Boudreau, Gary, Sediq, Akram Bin, Abou-zeid, Hatem, Wang, Xianbin&IEEE Transactions on Mobile Computing &2019 \\ \hline
S72&Online Reinforcement Learning for Beam Tracking and Rate Adaptation in Millimeter-wave Systems&Krunz, Marwan, Aykin, Irmak, Sarkar, Sopan, Akgun, Berk&IEEE Access &2023 \\ \hline
S73&Deep learning coordinated beamforming for highly-mobile millimeter wave systems&Alkhateeb, Ahmed, Alex, Sam, Varkey, Paul, Li, Ying, Qu, Qi, Tujkovic, Djordje&IEEE Transactions on Mobile Computing &2018 \\ \hline
S74&A deep learning framework for beam selection and power control in massive MIMO-millimeter-wave communications&Nguyen, Ti Ti, Nguyen, Kim-Khoa&IEEE Transactions on Wireless Communications&2022 \\ \hline
S75&A deep learning approach to location-and orientation-aided 3d beam selection for mmwave communications&Rezaie, Sajad, De Carvalho, Elisabeth, Manchn, Carles Navarro&IEEE Transactions on Wireless Communications&2022 \\ \hline
S76&Deep learning enabled optimization of downlink beamforming under per-antenna power constraints: Algorithms and experimental demonstration&Zhang, Juping, Xia, Wenchao, You, Minglei, Zheng, Gan, Lambotharan, Sangarapillai, Wong, Kai-Kit&IEEE Transactions on Wireless Communications&2020 \\ \hline
S77&A Reinforcement Learning Approach for Energy Efficient Beamforming in NOMA Systems&Liu, Yuqin, Zhong, Ruikang, Jaber, Mona&IEEE GLOBECOM&2022 \\ \hline
S78&Multi-agent deep reinforcement learning for distributed handover management in dense mmWave networks&Sana, Mohamed, De Domenico, Antonio, Strinati, Emilio Calvanese, Clemente, Antonio&IEEE International Conference on Acoustics, SpeechI and Signal Processing &2020 \\ \hline
S79&Efficient codebook-based beamforming algorithm for millimeter-wave massive MIMO systems&Chen, Jung-Chieh&IEEE Transactions on Vehicular Technology&2017 \\ \hline
S80&Clustering-based codebook design for MIMO communication system&Jiang, Jing, Wang, Xiaojing, Sidhu, Guftaar Ahmad Sardar, Zhen, Li, Gao, Runchen&IEEE International Conference on Communications&2019 \\ \hline
S81&Trainable projected gradient detector for massive overloaded MIMO channels: Data-driven tuning approach&Takabe, Satoshi, Imanishi, Masayuki, Wadayama, Tadashi, Hayakawa, Ryo, Hayashi, Kazunori&IEEE Access&2019 \\ \hline
S82&Machine learning-based beamforming in K-user MISO interference channels&Kwon, Hyung Jun, Lee, Jung Hoon, Choi, Wan&IEEE Access&2021 \\ \hline
S83&Deep learning for distributed channel feedback and multiuser precoding in FDD massive MIMO&Sohrabi, Foad, Attiah, Kareem M, Yu, Wei&IEEE Transactions on Wireless Communications&2021 \\ \hline
S84&On Assessing Vulnerabilities of the 5G Networks to Adversarial Examples&Zolotukhin, Mikhail, Miraghaei, Parsa, Zhang, Di, Ha&IEEE Access&2022 \\ \hline
S85&mmspy: Spying phone calls using mmwave radars&Basak, Suryoday, Gowda, Mahanth&IEEE Symposium on Security and Privacy&2022 \\ \hline
S86&mmTrack: Passive multi-person localization using commodity millimeter wave radio&Wu, Chenshu, Zhang, Feng, Wang, Beibei, Liu, KJ Ray& IEEE INFOCOM&2020 \\ \hline
S87&m-activity: Accurate and real-time human activity recognition via millimeter wave radar&Wang, Yuheng, Liu, Haipeng, Cui, Kening, Zhou, Anfu, Li, Wensheng, Ma, Huadong& IEEE International Conference on Acoustics, Speech and Signal Processing&2021 \\ \hline
S88&EarFisher: Detecting Wireless Eavesdroppers by Stimulating and Sensing Memory (EMR)&Shen, Cheng, Huang, Jun&USENIX Symposium on Networked Systems Design and Implementation&2021 \\ \hline
S89&Deep reinforcement learning based blind mmwave MIMO beam alignment&Raj, Vishnu, Nayak, Nancy, Kalyani, Sheetal&IEEE Transactions on Wireless Communications&2022 \\ \hline
S90&Beyond Codebook-Based Analog Beamforming at mmWave: Compressed Sensing and Machine Learning Methods&Pezeshki, H., Massoli, F.V., Behboodi, A., Yoo, T., Kannan, A., Boroujeni, M.T., Li, Q., Luo, T. and Soriaga, J.B&IEEE GLOBECOM&2022 \\ \hline
S91&Learning and data-driven beam selection for mmWave communications: An angle of arrival-based approach&Antn-Haro, Carles, Mestre, Xavier&IEEE Access &2019 \\ \hline
S92&Physical-layer security via distributed beamforming in the presence of adversaries with unknown locations&Savas, Yagiz, Hashemi, Abolfazl, Vinod, Abraham P, Sadler, Brian M, Topcu, Ufuk&IEEE International Conference on Acoustics, Speech and Signal Processing&2021 \\ \hline
S93&Channel estimation for cell-free mmWave massive MIMO through deep learning&Jin, Yu, Zhang, Jiayi, Jin, Shi, Ai, Bo&IEEE Transactions on Vehicular Technology&2019 \\ \hline
\hline
S94 & Evaluating adversarial evasion attacks in the context of wireless communications & Flowers, Bryse, et al. & IEEE Transactions on Information Forensics and Security & 2019 \\
\hline
S95 & Robust adversarial attacks against DNN-based wireless communication systems & Bahramali, Alireza, et al. & ACM Symposium on Computer and Communications Security & 2021  \\
\hline
S96 & Poison Neural Network-Based mmWave Beam Selection and Detoxification With Machine Unlearning & Zhang, Zhengming, et al. & IEEE Transactions on Communications & 2022  \\
\hline
S97 & Data poisoning attacks and defenses in dynamic crowdsourcing with online data quality learning & Zhao, Yuxi, et al. & IEEE Transactions on Mobile Computing & 2021 \\
\hline
S98 & Backdoor federated learning-based mmWave beam selection & Zhang, Zhengming, et al. & IEEE Transactions on Communications & 2022  \\
\hline
S99 & A lightweight auction framework for spectrum allocation with strong security guarantees & Cheng, Ke, et al. & IEEE INFOCOM & 2020  \\
\hline
S100 & Bayesian Inference-assisted Machine Learning for Near Real-Time Jamming Detection and Classification in 5G New Radio (NR) & Jere, Shashank, et al. & IEEE Transactions on Wireless Communications & 2023  \\
\hline
S101 & Securing large-scale d2d networks using covert communication and friendly jamming & Feng, Shaohan, et al. & IEEE Transactions on Wireless Communications & 2023  \\
\hline
S102 & A Defensive Strategy Against Beam Training Attack in 5G mmWave Networks for Manufacturing & Dinh-Van, Son, et al. & IEEE Transactions on Information Forensics and Security & 2023  \\
\hline
S103 & A trust-centric privacy-preserving blockchain for dynamic spectrum management in IoT networks & Ye, Jingwei, et al. & IEEE Internet of Things Journal & 2022  \\
\hline
S104 & An efficient privacy preserving spectrum sharing framework for internet of things & Wang, Xiaoyan, et al. & IEEE Access & 2020  \\
\hline
S105 & Detection and localization of the eavesdropper in MIMO systems & Ning, Lina, et al. & IEEE Access & 2020  \\
\hline
S106 & Secrecy Rate Maximization in THz-Aided Heterogeneous Networks: A Deep Reinforcement Learning Approach & Sharma, Himanshu, et al. & IEEE Transactions on Vehicular Technology & 2023  \\
\hline
S107 & On mitigation of pilot spoofing attack & Tugnait, Jitendra K & IEEE Intl. Conf. on Acoustics, Speech and Signal Processing & 2017  \\
\hline
S108 & Physical layer spoofing attack detection in MmWave massive MIMO 5G networks & Li, Weiwei, et al. & IEEE Access & 2021  \\
\hline
S109 & Exploiting beam features for spoofing attack detection in mmWave 60-GHz IEEE 802.11 ad networks & Wang, Ning, et al. & IEEE Transactions on Wireless Communications & 2021  \\
\hline
S110 & Concurrent Spoofing-Jamming Attack in Massive MIMO Systems with a Full-Duplex Multi-Antenna Eavesdropper & Alageli, Mahmoud, et al. & IEEE Transactions on Vehicular Technology & 2023  \\
\hline
\end{longtable}

% \bibliographystyle{ieeetr}
% \bibliography{reviewedstudies}
